# Supplementary material for: Two-Photon Excitation Sets Limit to Entangled Photon Pair Generation from Quantum Emitters
Source: arXiv:2205.03390 ancillary file (2022-11-11)
Supplement: Supplementary file 1 [file Supplement_Impact_TPE.pdf]

# Supplement: Two-Photon Excitation Sets Limit to Entangled Photon Pair Generation from Quantum Emitters


T. Seidelmann,[1,*] C. Schimpf,[2] T. K. Bracht,[3] M. Cosacchi,[1] A. Vagov,[1] A. Rastelli,[2] D. E. Reiter,[3,†] and V. M. Axt[1]

[1] *Lehrstuhl für Theoretische Physik III, Universität Bayreuth, 95440 Bayreuth, Germany*
[2] *Institute of Semiconductor and Solid State Physics, Johannes Kepler University Linz, 4040 Linz, Austria*
[3] *Institut für Festkörpertheorie, Universität Münster, 48149 Münster, Germany*


## A. THEORETICAL MODEL, DENSITY MATRIX AND CONCURRENCE

### I. Optically excited quantum dot and system dynamics

In this section, we provide more details on the theoretical model and the determination of the two-photon density matrix and its corresponding degree of entanglement as measured by the concurrence.

In our simulations, we consider the biexciton-exciton cascade of a quantum dot (QD) excited by a two-photon resonant Gaussian laser pulse. In a frame co-rotating with the laser frequency $\omega_\mathrm{L}$, the Hamiltonian $\hat{H}_\text{QD-L}$, describing the interaction of the QD with the applied laser pulse, is given by

$$\hat{H}_\text{QD-L} = \left(\Delta_\mathrm{XL} + \frac{\delta}{2}\right)|X_\mathrm{H}\rangle\langle X_\mathrm{H}| + \left(\Delta_\mathrm{XL} - \frac{\delta}{2}\right)|X_\mathrm{V}\rangle\langle X_\mathrm{V}| + (2\Delta_\mathrm{XL} - E_\mathrm{B})\,|B\rangle\langle B| - \frac{\hbar}{2}\,\Omega(t)\left(\hat{\sigma}_\mathrm{L} + \hat{\sigma}_\mathrm{L}^\dagger\right) \tag{A1}$$

Here, $\delta = \hbar\,(\omega_\mathrm{H} - \omega_\mathrm{V})$ denotes the fine-structure splitting between the energies $\hbar\omega_\mathrm{H}$ and $\hbar\omega_\mathrm{V}$ of the orthogonally polarized exciton states $|X_\mathrm{H}\rangle$ and $|X_\mathrm{V}\rangle$, which couple to horizontally and vertically polarized light, respectively, and the exciton-laser detuning $\Delta_\mathrm{XL} = \hbar\,(\omega_\mathrm{X} - \omega_\mathrm{L})$ is the energetic difference between the mean exciton energy $\hbar\omega_\mathrm{X} = \hbar\,(\omega_\mathrm{H} + \omega_\mathrm{V})\,/2$ and the laser. The energy of the ground state $|G\rangle$ is used as the zero of the energy scale and the biexciton binding energy $E_\mathrm{B}$ lowers the energy of the biexciton state $|B\rangle$ compared to the sum of both exciton energies.

In this article, we assume a Gaussian pulse shape with (real) envelope

$$\Omega(t) = \sqrt{\frac{4\ln(2)}{\pi}}\,\frac{\Theta}{\Delta_\mathrm{FWHM}}\,\exp\left[-4\ln(2)\left(\frac{t - t_\mathrm{L}}{\Delta_\mathrm{FWHM}}\right)^2\right] \tag{A2}$$

where $\Theta$ is the (one-photon resonant) pulse area and $t_\mathrm{L}$ is the time of the pulse maximum. The duration in time of this Gaussian pulse is characterized by its full-width-at-half-maximum (FWHM) $\Delta_\mathrm{FWHM}$. In order to achieve a two-photon resonant excitation of the biexciton state, the laser frequency is set to half of the ground state-to-biexciton transition energy, i.e., $\Delta_\mathrm{XL} = E_\mathrm{B}/2$ and a linear laser polarization is considered. In the basis spanned by the horizontal $(H)$ and vertical $(V)$ polarization associated with the two orthogonally polarized exciton states, the laser polarization can be described by

$$\hat{\sigma}_\mathrm{L} = \alpha_H\hat{\sigma}_H + \alpha_V\hat{\sigma}_V \tag{A3}$$

where the transition operators

$$\hat{\sigma}_{H/V} = |G\rangle\langle X_\mathrm{H/V}| + |X_\mathrm{H/V}\rangle\langle B| \tag{A4}$$

describe QD transitions that couple to horizontally/vertically polarized light and the coefficient $\alpha_{H/V} \in \mathbb{R}$ is the component of the laser polarization in $H/V$ direction.

The transitions between QD states accompanied by photon emission are modeled as a radiative decay with rates $\Gamma$ and incorporated in the model via Lindblad operators [1]

$$\mathcal{L}_{\hat{O},\Gamma}\hat{\rho} = \frac{\Gamma}{2}\left(2\hat{O}\hat{\rho}\hat{O}^\dagger - \hat{O}^\dagger\hat{O}\hat{\rho} - \hat{\rho}\hat{O}^\dagger\hat{O}\right), \tag{A5}$$


* Corresponding author: tim.seidelmann@uni-bayreuth.de
† Current address: Condensed Matter Theory, Department of Physics, TU Dortmund, 44221 Dortmund, Germany

acting on the statistical operator $\hat{\rho}$ of the QD system, where the operator $\hat{O}$ describes the relevant QD transition. Due to the optical selection rules, we consider the four operators $\mathcal{L}_{|G\rangle\langle X_\mathrm{H}|,\gamma_\mathrm{X}}$, $\mathcal{L}_{|G\rangle\langle X_\mathrm{V}|,\gamma_\mathrm{X}}$, $\mathcal{L}_{|X_\mathrm{H}\rangle\langle B|,\frac{\gamma_\mathrm{B}}{2}}$, and $\mathcal{L}_{|X_\mathrm{V}\rangle\langle B|,\frac{\gamma_\mathrm{B}}{2}}$, where $\gamma_\mathrm{B}$ ($\gamma_\mathrm{X}$) denotes the decay rate of the biexciton (exciton) state.

The dynamics of the statistical operator of the system $\hat{\rho}$ is governed by the Liouville-von Neumann equation

$$\frac{\mathrm{d}}{\mathrm{d}t}\hat{\rho} = \mathcal{L}\hat{\rho} := -\frac{i}{\hbar}\left[\hat{H},\hat{\rho}\right] + \sum_{\ell=H,V}\left\{\mathcal{L}_{|G\rangle\langle X_\ell|,\gamma_\mathrm{X}} + \mathcal{L}_{|X_\ell\rangle\langle B|,\frac{\gamma_\mathrm{B}}{2}}\right\}\hat{\rho}, \tag{A6}$$

where $[\hat{A},\hat{B}]$ denotes the commutator of two operators $\hat{A}$ and $\hat{B}$. This equation is numerically solved using its formal solution

$$\hat{\rho}(t) = \mathcal{P}_{0\to t}\left[\hat{\rho}(0)\right] := \hat{T}\exp\left[\int_0^t \mathrm{d}t'\mathcal{L}(t')\right]\hat{\rho}(0) \tag{A7}$$

where $\mathcal{P}_{0\to t}$ denotes a formal propagator in time, $\hat{T}$ is the time-ordering operator, and we assume the QD to be initially in its ground state.

In order to perform studies using a two-photon resonant $\pi$-pulse to excite the biexciton state, the corresponding pulse area $\Theta$ of the Gaussian pulse has to be determined. This is done numerically for each individual calculation by optimizing $\Theta$ to obtain the maximum biexciton occupation during the real-time dynamics. In the situation considered here where $\Omega(t)/E_\mathrm{B}$ is a small quantity, a first approximation for this value

$$\Theta \approx \sqrt{\frac{E_\mathrm{B}\,\Delta_\mathrm{FWHM}}{\hbar\sqrt{2\pi\ln 2}}}\,\pi \tag{A8}$$

can be obtained by performing a Schrieffer-Wolff transformation [2, 3] on the QD-laser Hamiltonian $\hat{H}_\mathrm{QD\text{-}L}$. In the actual simulations, the numerically determined optimal value for $\Theta$ is typically 5...20% higher, depending on the FWHM $\Delta_\mathrm{FWHM}$.

## II. Reconstructed two-photon density matrix

In standard experiments, the emitted photon state is reconstructed using quantum state tomography [4], a well-established scheme that is based on polarization-resolved two-time correlation measurements. The signal obtained in these type of measurements are proportional to two-time correlation functions containing electric field operators at different times. Since electronic transitions in the QD four-level system are the source for the emitted field, the electric field operators are in turn proportional to the QD transition operators $\hat{\sigma}_\mathrm{H/V}$ and the relevant correlation functions can be theoretically calculated by evaluating the correlation functions

$$G^{(2)}_{jk,\ell m}(t,\tau) = \left\langle \hat{\sigma}^\dagger_j(t)\hat{\sigma}^\dagger_k(t+\tau)\hat{\sigma}_m(t+\tau)\hat{\sigma}_\ell(t)\right\rangle, \tag{A9}$$

where $\{j,k,\ell,m\}\in\{H,V\}$. The time $t$ denotes the time of the first detection event and $\tau$ is the delay time until a subsequent second one.

In an actual measurement, one always averages over both times, the real time $t$, as well as the delay time $\tau$. While the integration interval for the real time $T_\mathrm{av}$ is extended over the complete decay process, different subsets of photon pairs can be selected by using different integration intervals $\tau_\mathrm{av}$ for the delay time [5]. For example, simultaneously emitted photon pairs are selected in the limit of a vanishing integration window $\tau_\mathrm{av}\to 0$. But there are always experimental limits to the time resolution down to 20-300 picoseconds, depending on the setup.

Furthermore, in application-oriented experiments, one aims to obtain the maximum photon yield, which corresponds to considering all emission events, i.e., the limit $\tau_\mathrm{av}\to\infty$ is used. Consequently, in our studies, the (normalized) two-photon density matrix $\rho^\mathrm{2p}$ is given by

$$\rho^\mathrm{2p}_{jk,\ell m} = \frac{\overline{G}^{(2)}_{jk,\ell m}}{\mathrm{Tr}\left\{\overline{G}^{(2)}\right\}} \tag{A10a}$$

$$\overline{G}^{(2)}_{jk,\ell m} = \lim_{T_\mathrm{av},\tau_\mathrm{av}\to\infty}\int_0^{T_\mathrm{av}}\mathrm{d}t\int_0^{\tau_\mathrm{av}}\mathrm{d}\tau\,G^{(2)}_{jk,\ell m}(t,\tau) \tag{A10b}$$

where, both integration intervals are considered in the limit of infinity. In our numerical calculations, these quantities are evaluated by re-writing Eq. (A9) in the Schrödinger picture [6]

$$G^{(2)}_{jk,\ell m}(t,\tau) = \left\langle \hat{\sigma}^\dagger_k \hat{\sigma}_m \mathcal{P}_{t\to t+\tau} \left[ \hat{\sigma}_\ell \mathcal{P}_{0\to t} \left[\hat{\rho}(0)\right] \hat{\sigma}^\dagger_j \right] \right\rangle \tag{A11}$$

### III. Degree of entanglement

The degree of entanglement associated with a given two-photon density matrix is quantified using the concurrence $C$, a well-established measure which has a one-to-one correspondence to the entanglement of formation [7]. The concurrence can be obtained directly form the two-photon density matrix $\rho^{2\mathrm{p}}$ by calculating the four (real and positive) eigenvalues $\lambda_j$ of the matrix

$$M = \rho^{2\mathrm{p}}\, T\, (\rho^{2\mathrm{p}})^*\, T, \tag{A12}$$

where $(\rho^{2\mathrm{p}})^*$ denotes the complex conjugated two-photon density matrix and $T$ is the anti-diagonal matrix with elements $\{-1,1,1,-1\}$. After sorting the eigenvalues in decreasing order, $\lambda_{j+1} \leq \lambda_j$, the concurrence is given as [4, 7, 8]:

$$C = \max\left\{0, \sqrt{\lambda_1} - \sqrt{\lambda_2} - \sqrt{\lambda_3} - \sqrt{\lambda_4}\right\}, \tag{A13}$$

A quite useful approximation for the concurrence is

$$C \approx 2\left(|\rho^{2\mathrm{p}}_{HH,VV}| - \rho^{2\mathrm{p}}_{HV,HV}\right). \tag{A14}$$

This expression is exactly fulfilled for a two-photon density matrix, that has the form

$$\rho^{2\mathrm{p}} = \begin{pmatrix} a & 0 & 0 & c \\ 0 & b & d & 0 \\ 0 & d^* & b & 0 \\ c^* & 0 & 0 & a' \end{pmatrix} \tag{A15}$$

in the basis $\{|HH\rangle, |HV\rangle, |VH\rangle, |VV\rangle\}$ where the parameters $a, a', b \in \mathbb{R}^+$, $c, d \in \mathbb{C}$ fulfill $a + a' + 2b = 1$ and $\sqrt{a\, a'} \geq |c| \geq b \geq |d|$. Thus, Eq. (A14) is a good approximation for the concurrence, if a two-photon density matrix is dominated by the elements $\rho^{2\mathrm{p}}_{HH,HH}$, $\rho^{2\mathrm{p}}_{VV,VV}$, and $\rho^{2\mathrm{p}}_{HH,VV}$, the condition $\rho^{2\mathrm{p}}_{HV,HV} = \rho^{2\mathrm{p}}_{VH,VH}$ is approximately fulfilled, and the 8 remaining coherences can be neglected. In our numerical simulations, we obtain density matrices of this kind for the considered parameter regime. Thus we use this approximate formula for the analytic calculations.

## B. INITIAL VALUE CALCULATIONS

In this section a brief derivation for the quantity $C_0$ is given, which represents the concurrence in the case of an initially prepared biexciton state.

Without an external laser the Hamiltonian describing the system reduces to

$$\hat{H}_0 := \frac{E_\mathrm{B} + \delta}{2} |X_\mathrm{H}\rangle\langle X_\mathrm{H}| + \frac{E_\mathrm{B} - \delta}{2} |X_\mathrm{V}\rangle\langle X_\mathrm{V}| \tag{B1}$$

in a frame rotating with the frequency $\omega_\mathrm{L} = \omega_\mathrm{X} - E_\mathrm{B}/(2\hbar)$. This Hamiltonian is of course diagonal in the basis $\{|G\rangle, |X_\mathrm{H}\rangle, |X_\mathrm{V}\rangle, |B\rangle\}$ and time-independent. Therefore, the formal solution of the Liouville-von Neumann equation

$$\frac{\mathrm{d}}{\mathrm{d}t}\hat{\rho} = \mathcal{L}_0\hat{\rho} := -\frac{i}{\hbar}\left[\hat{H}_0, \hat{\rho}\right] + \sum_{\ell=H,V} \left\{ \mathcal{L}_{|G\rangle\langle X_\ell|, \gamma_\mathrm{X}} + \mathcal{L}_{|X_\ell\rangle\langle B|, \frac{\gamma_\mathrm{B}}{2}} \right\} \hat{\rho}, \tag{B2}$$

for the statistical operator $\hat{\rho}$ is given by

$$\hat{\rho}(t) = \mathcal{P}^{(0)}_{t_0\to t}[\hat{\rho}(t_0)] := \exp[\mathcal{L}_0\,(t - t_0)]\hat{\rho}(t_0). \tag{B3}$$

where $\mathcal{L}_0$ is a time-independent operator in Liouville space and $\mathcal{P}^{(0)}_{t_0\to t}$ the corresponding formal propagator for the statistical operator. In particular one obtains

$$\langle B|\mathcal{P}^{(0)}_{t_0\to t}[|B\rangle\langle B|]|B\rangle = e^{-\gamma_{\rm B}\,(t-t_0)} \tag{B4a}$$

$$\langle X_m|\mathcal{P}^{(0)}_{t_0\to t}[|X_\ell\rangle\langle X_j|]|X_k\rangle = \delta_{jk}\delta_{\ell m}e^{-[\gamma_{\rm X}+i(E_\ell-E_j)/\hbar](t-t_0)} \tag{B4b}$$

where $j,k,\ell,m \in \{H,V\}$ and $E_{H/V} = (E_{\rm B}\pm\delta)/2$. In order to calculate the reconstructed two-photon density matrix, integrated two-time correlation functions have to be evaluated. In the Schrödinger picture Eq. (A10b) can be reformulated as

$$\overline{G}^{(2)}_{jk,\ell m} = \int\limits_0^\infty {\rm d}t \int\limits_0^\infty {\rm d}\tau\, G^{(2)}_{jk,\ell m}(t,\tau) = \int\limits_0^\infty {\rm d}t \int\limits_0^\infty {\rm d}\tau\, {\rm Tr}\left\{\hat\sigma^\dagger_k\hat\sigma_m\mathcal{P}^{(0)}_{t\to t+\tau}\left[\hat\sigma_\ell\mathcal{P}^{(0)}_{0\to t}[\hat\rho(0)]\hat\sigma^\dagger_j\right]\right\} \tag{B5}$$

Note that in a time evolution governed by the propagator $\mathcal{P}^{(0)}_{t_0\to t}$ the system can only relax towards its ground state $|G\rangle$ and no excitation is ever transferred to higher excited states, i.e., no excitation is transferred from the ground state $|G\rangle$ (exciton state $|X_j\rangle$) towards an exciton state $|X_j\rangle$ (biexciton state $|B\rangle$). Therefore $\overline{G}^{(2)}_{jk,\ell m}$ is only nonzero if the system is in the biexciton at the time $t$ when the first pair of transition operators is applied. This is a direct consequence of the considered system, where the interaction with the field modes can be modeled as radiative decay. Thus, the re-absorption of emitted photons cannot occur. In other systems, e.g., when the QD is embedded inside a high-quality microcavity, photons inside the cavity are likely to be re-absorbed by the QD, leading to an oscillating biexciton occupation. Furthermore, since the operator $\mathcal{L}_0$ is time-independent, the propagator depends only on a time difference, i.e., $\mathcal{P}^{(0)}_{t_0\to t} = \mathcal{P}^{(0)}_{0\to t-t_0}$. Starting with an initially prepared biexciton state, i.e., $\hat\rho(0) = |B\rangle\langle B|$, and inserting the formal propagation (B4) one arrives at

$$\begin{aligned}\overline{G}^{(2)}_{jk,\ell m} &= \int\limits_0^\infty {\rm d}t \int\limits_0^\infty {\rm d}\tau\, {\rm Tr}\left\{\hat\sigma^\dagger_k\hat\sigma_m\mathcal{P}^{(0)}_{t\to t+\tau}\left[|X_\ell\rangle\langle B|\mathcal{P}^{(0)}_{0\to t}\left[|B\rangle\langle B|\right]|B\rangle\langle X_j|\right]\right\}\\ &= \int\limits_0^\infty {\rm d}t \int\limits_0^\infty {\rm d}\tau\, {\rm Tr}\left\{\hat\sigma^\dagger_k\hat\sigma_m\mathcal{P}^{(0)}_{0\to\tau}\left[e^{-\gamma_{\rm B}\,t}|X_\ell\rangle\langle X_j|\right]\right\} = \frac{1}{\gamma_{\rm B}}\int\limits_0^\infty {\rm d}\tau\, {\rm Tr}\left\{\hat\sigma^\dagger_k\hat\sigma_m\mathcal{P}^{(0)}_{0\to\tau}\left[|X_\ell\rangle\langle X_j|\right]\right\}\\ &= \frac{1}{\gamma_{\rm B}}\int\limits_0^\infty {\rm d}\tau\, \delta_{jk}\delta_{\ell m}e^{-[\gamma_{\rm X}+i(E_\ell-E_j)/\hbar]\tau} = \frac{1}{\gamma_{\rm B}}\delta_{jk}\delta_{\ell m}\frac{1}{\gamma_{\rm X}+i(E_\ell-E_j)/\hbar}\end{aligned} \tag{B6}$$

From these quantities the elements of the two-photon density matrix are obtained according to Eq. (A10a). As expected one finds only four nonzero elements

$$\rho^{\rm 2p}_{HH,HH} = \frac{1}{2} = \rho^{\rm 2p}_{VV,VV} \tag{B7a}$$

$$\rho^{\rm 2p}_{HH,VV} = \frac{1}{2}\frac{1}{1-i\frac{\delta}{\hbar\gamma_{\rm X}}} = \left(\rho^{\rm 2p}_{VV,HH}\right)^* \tag{B7b}$$

In this situation, the definition of the concurrence given in Eqs. (A12) and (A13) reduces to

$$C = 2|\rho^{\rm 2p}_{HH,VV}| = \frac{1}{\sqrt{1+\left(\frac{\delta}{\hbar\gamma_{\rm X}}\right)^2}} =: C_0(\gamma_{\rm X},\delta) \tag{B8}$$

## C. CALCULATIONS WITH FINITE FWHM

In this section a brief derivation of the analytic approximation for the concurrence in Eq. (6) in the main text is given, which takes into account the impact of a finite pulse duration in a two-photon resonant excitation scheme. Here, the calculation is performed for an arbitrary linear laser polarization. Special cases and interpretations are discussed in the following Sections D, E and G.

The basic idea for the analytic estimate is inspired by the initial value calculation in the previous section. We consider a short time interval centered around the time of the pulse maximum and assume that the Gaussian pulse only interacts with the QD during this time. Additionally, we replace the time-dependent shape of the pulse by an effective constant driving. Based on these main steps and some further assumptions, in particular that $\gamma_{\mathrm{B}}\Delta_{\mathrm{FWHM}}/2$ and $\gamma_{\mathrm{X}}\Delta_{\mathrm{FWHM}}$ are small quantities, we rework the calculations for the concurrence.

### I. Effective model with constant driving

For the effective model, we define a time interval with length $F$ centered around the time of the pulse maximum and assume that the Gaussian pulse only interacts with the QD in this interval $t \in [t_{\mathrm{L}} - F/2, t_{\mathrm{L}} + F/2]$. Additionally, we replace the time-dependent amplitude of the laser pulse $\Omega(t)$ by an effective constant driving strength $\Omega_{\mathrm{eff}}$. Furthermore, the fine-structure splitting between the excitons is neglected during the time interval $F$ since a splitting $\delta \ll E_{\mathrm{B}}$ has hardly any impact on the two-photon resonant excitation scheme. Because the two-photon process exciting the QD from the ground state towards the biexciton state is a second order process and scales with $\Omega^2(t)$, it is plausible to assume, that this interval starts at the time $\Delta_{\mathrm{FWHM}}/2$ before the pulse maximum, since $\Omega^2(t_{\mathrm{L}} - \Delta_{\mathrm{FWHM}}/2) \leq \Omega^2(t_{\mathrm{L}})/4$. Thus we set $F = \Delta_{\mathrm{FWHM}}$ for the moment. An effective constant driving $\Omega_{\mathrm{eff}}$ should fulfill the relation

$$\int\limits_{t_{\mathrm{L}}-F/2}^{t_{\mathrm{L}}+F/2} \mathrm{d}t\, \Omega(t) = \int\limits_{t_{\mathrm{L}}-F/2}^{t_{\mathrm{L}}+F/2} \mathrm{d}t\, \sqrt{\frac{4\ln(2)}{\pi}} \frac{\Theta}{\Delta_{\mathrm{FWHM}}} e^{-4\ln(2)\left(\frac{t-t_{\mathrm{L}}}{\Delta_{\mathrm{FWHM}}}\right)^2} = \int\limits_{t_{\mathrm{L}}-F/2}^{t_{\mathrm{L}}+F/2} \mathrm{d}t\, \Omega_{\mathrm{eff}} = F\, \Omega_{\mathrm{eff}} \tag{C1}$$

With the choice $F = \Delta_{\mathrm{FWHM}}$ one obtains

$$\Omega_{\mathrm{eff}} \approx 0.81 \sqrt{\frac{4\ln 2}{\pi}} \frac{\Theta}{\Delta_{\mathrm{FWHM}}} \tag{C2}$$

Based on these assumptions, the effective Hamiltonian for a laser pulse with an arbitrary linear polarization is given by

$$\hat{H}^{\mathrm{eff}}_{\text{QD-L}} = \begin{cases} \hat{H}_1 & , t \in [t_{\mathrm{L}} - F/2, t_{\mathrm{L}} + F/2] \\ \hat{H}_0 & , \text{otherwise} \end{cases} \tag{C3a}$$

$$\hat{H}_1 = \frac{E_{\mathrm{B}}}{2} \left(|X_{\mathrm{H}}\rangle\langle X_{\mathrm{H}}| + |X_{\mathrm{V}}\rangle\langle X_{\mathrm{V}}|\right) + \frac{\hbar}{2}\, \Omega_{\mathrm{eff}} \left(\hat{\sigma}_{\mathrm{L}} + \hat{\sigma}^{\dagger}_{\mathrm{L}}\right) \tag{C3b}$$

$$\hat{\sigma}_{\mathrm{L}} = \alpha_H \hat{\sigma}_H + \alpha_V \hat{\sigma}_V \tag{C3c}$$

in the frame co-rotating with the laser frequency $\omega_{\mathrm{L}}$ set to the two-photon resonance. The linear polarization of the laser is defined by the (real) coefficients $\alpha_H$ and $\alpha_V$ which fulfill $\alpha_H^2 + \alpha_V^2 = 1$ and represent the component in $H$ and $V$ polarization, respectively. The four energy eigenstates of $\hat{H}_1$ are given by

$$|U\rangle = c\left(|G\rangle + |B\rangle\right) + \sqrt{2}\tilde{c}\left(\alpha_H |X_{\mathrm{H}}\rangle + \alpha_V |X_{\mathrm{V}}\rangle\right) \tag{C4a}$$

$$|M\rangle = \alpha_V |X_{\mathrm{H}}\rangle - \alpha_H |X_{\mathrm{V}}\rangle \tag{C4b}$$

$$|N\rangle = \frac{1}{\sqrt{2}}\left(|G\rangle - |B\rangle\right) \tag{C4c}$$

$$|L\rangle = \tilde{c}\left(|G\rangle + |B\rangle\right) - \sqrt{2}c\left(\alpha_H |X_{\mathrm{H}}\rangle + \alpha_V |X_{\mathrm{V}}\rangle\right) \tag{C4d}$$

with coefficients

$$c = \frac{\hbar\Omega_{\mathrm{eff}}}{\sqrt{2(\hbar\Omega_{\mathrm{eff}})^2 + 4E_{\mathrm{U}}^2}};\ \tilde{c} = \sqrt{\frac{1}{2} - c^2} \tag{C5}$$

The corresponding eigenenergies

$$E_{\mathrm{U}} = \frac{1}{4}\left(E_{\mathrm{B}} + \sqrt{E_{\mathrm{B}}^2 + 8(\hbar\Omega_{\mathrm{eff}})^2}\right) \tag{C6a}$$

$$E_{\mathrm{M}} = \frac{E_{\mathrm{B}}}{2} \tag{C6b}$$

$$E_{\mathrm{N}} = 0 \tag{C6c}$$

$$E_{\mathrm{L}} = \frac{1}{4}\left(E_{\mathrm{B}} - \sqrt{E_{\mathrm{B}}^2 + 8(\hbar\Omega_{\mathrm{eff}})^2}\right) \tag{C6d}$$

are independent of the laser polarization, i.e., independent of $\alpha_{H/V}$.

### II. Approximate time dynamics in the effective model

Without radiative decay, the time evolution of the statistical operator for times $t, t_0 \in [t_\mathrm{L} - \Delta_\mathrm{FWHM}/2, t_\mathrm{L} + \Delta_\mathrm{FWHM}/2]$ in the effective model is determined by

$$\hat{\rho}(t) = \mathcal{P}^{(1)}_{t_0\to t}\hat{\rho}(t_0)] := \exp[\mathcal{L}_1\,(t-t_0)]\hat{\rho}(t_0) \tag{C7a}$$

$$\mathcal{L}_1\hat{\rho} := -\frac{i}{\hbar}\left[\hat{H}_1, \hat{\rho}\right] \tag{C7b}$$

Combining the expression (C2) with the estimate for the optimal pulse area in Eq. (A8), we realize that $(\hbar\Omega_\mathrm{eff})^2/E_\mathrm{B}^2 \ll 1$ for our parameters and, thus, the coefficients $c$ and $\tilde{c}$ fulfill

$$\tilde{c}^2 \approx \frac{1}{2};\ \left(\frac{c}{\tilde{c}}\right)^2 \ll 1 \tag{C8}$$

Consequently, the two eigenstates $|N\rangle$ and $|L\rangle$ are approximately an equal admixture of ground and biexciton state, i.e., $|N/L\rangle \approx (|G\rangle \mp |B\rangle)/\sqrt{2}$. Therefore, the time evolution after an initially prepared ground state is mainly described by these two eigenstates and the time evolution of the biexciton state can be approximated as

$$\rho_\mathrm{BB}(t) = \langle B|\mathcal{P}^{(1)}_{t_0\to t}[|G\rangle\langle G|]|B\rangle \approx \frac{1}{2}\left[1-\cos\left(E_\mathrm{L}\,(t-t_0)/\hbar\right)\right] \tag{C9}$$

Taking into account radiative decay described by the Lindblad operators $\mathcal{L}_{|X_\mathrm{H}\rangle\langle B|,\frac{\gamma_\mathrm{B}}{2}}$ and $\mathcal{L}_{|X_\mathrm{V}\rangle\langle B|,\frac{\gamma_\mathrm{B}}{2}}$, both eigenstates $|N\rangle$ and $|L\rangle$ should decay with the rate $\gamma_\mathrm{B}/2$, since both are close to an equal admixture of $|G\rangle$ and $|B\rangle$. In the situation $(\hbar\Omega_\mathrm{eff})^2/E_\mathrm{B}^2 \ll 1$, one obtains

$$\frac{E_\mathrm{U}-E_\mathrm{M}}{\hbar} = \frac{|E_\mathrm{L}|}{\hbar} \approx \frac{\hbar\Omega_\mathrm{eff}^2}{E_\mathrm{B}} = 0.81^2\,\frac{2\sqrt{2\pi\ln 2}}{\Delta_\mathrm{FWHM}} \tag{C10}$$

by inserting Eqs. (A8) and (C2). Furthermore, as stated in Section A I, we observed that in the presence of radiative decay, the optimal pulse area is actually around 10% higher than estimated in Eq. (A8). Taking this factor into account, Eq. (C10) can be (nicely) approximated as

$$\frac{E_\mathrm{U}-E_\mathrm{M}}{\hbar} = \frac{|E_\mathrm{L}|}{\hbar} \approx \frac{\pi}{\Delta_\mathrm{FWHM}} \tag{C11}$$

This also means that, the energetic splitting between the two upper dressed states $E_\mathrm{S}$ (cf., Fig. C1), which is always identical to the energetic splitting between the two lower ones, is approximately

$$E_\mathrm{S} = E_\mathrm{U} - E_\mathrm{M} = E_\mathrm{N} - E_\mathrm{L} \approx \frac{\hbar\pi}{\Delta_\mathrm{FWHM}} \tag{C12}$$

Altogether, the biexciton occupation during the effective pulse interval is therefore estimated as

$$\rho_\mathrm{BB}(t) = \langle B|\mathcal{P}^{(2)}_{t_0\to t}[|G\rangle\langle G|]|B\rangle \approx \frac{1}{2}\left[1-\cos\left(\frac{\pi\,(t-t_0)}{\Delta_\mathrm{FWHM}}\right)\right]e^{-\gamma_\mathrm{B}(t-t_0)/2} \tag{C13a}$$

$$\mathcal{P}^{(2)}_{t_0\to t}[\hat{\rho}(t_0)] := \exp[\mathcal{L}_2\,(t-t_0)]\hat{\rho}(t_0) \tag{C13b}$$

$$\mathcal{L}_2\hat{\rho} := -\frac{i}{\hbar}\left[\hat{H}_1,\hat{\rho}\right] + \sum_{\ell=H,V}\left\{\mathcal{L}_{|G\rangle\langle X_\ell|,\gamma_\mathrm{X}} + \mathcal{L}_{|X_\ell\rangle\langle B|,\frac{\gamma_\mathrm{B}}{2}}\right\}\hat{\rho} \tag{C13c}$$

Note that these formulas are independent of the laser polarization. Any linear laser polarization will result in this estimate for the biexciton occupation during the laser pulse.

Figure C2 depicts the comparison of the effective model, where Eq. (C13a) is used to describe the biexciton occupation during the time interval $t \in [t_\mathrm{L} - \Delta_\mathrm{FWHM}/2, t_\mathrm{L} + \Delta_\mathrm{FWHM}/2]$, with the numerical data. For our purposes, the estimated dynamics agrees reasonably well with the numerically obtained dynamics, justifying the choice $F = \Delta_\mathrm{FWHM}$ and the use of the effective model.

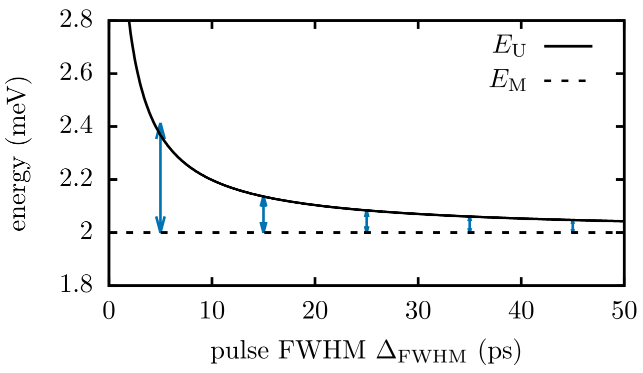


FIG. C1. Dressed state energies $E_{\mathrm{U}}$ and $E_{\mathrm{M}}$ as function of the FWHM $\Delta_{\mathrm{FWHM}}$ for an effective driving strength $\Omega_{\mathrm{eff}}$ according to Eq. (C2). In accordance with our numerical observation, the optimal pulse area $\Theta$ is set to 1.1 times the value predicted by the Schrieffer-Wolff transformation in Eq. (A8). Blue double-headed arrows indicate the energetic splitting $E_{\mathrm{S}} = \hbar\pi/\Delta_{\mathrm{FWHM}}$.

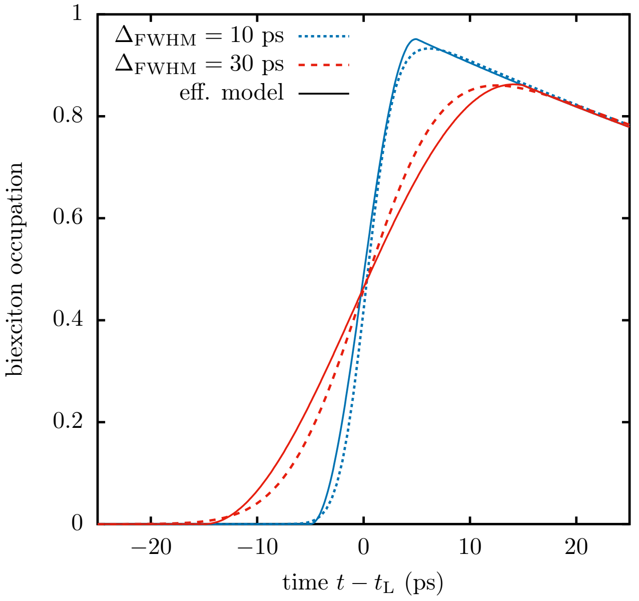


FIG. C2. Biexciton occupation obtained from the numerical simulations compared to results according to Eq. (C13a) and the effective Hamiltonian for two different pulse FWHMs $\Delta_{\mathrm{FWHM}}$.

In the following, we also need an approximation for the propagation of an exciton occupation or coherence during the time window of the laser pulse after the emission of a first biexciton photon. Employing similar approximations, in particular, $|U/M\rangle \approx \alpha_{H/V}|X_{\mathrm{H}}\rangle \pm \alpha_{V/H}|X_{\mathrm{V}}\rangle$ and Eq. (C11), one obtains

$$\langle X_j|\mathcal{P}^{(1)}_{t_0\to t}[|X_j\rangle\langle X_j|]|X_j\rangle \approx 1 + 2\alpha_H^2\alpha_V^2\left[\cos\left(\frac{\pi(t-t_0)}{\Delta_{\mathrm{FWHM}}}\right) - 1\right] \tag{C14a}$$

$$\langle X_\ell|\mathcal{P}^{(1)}_{t_0\to t}[|X_j\rangle\langle X_j|]|X_\ell\rangle \approx 2\alpha_H^2\alpha_V^2\left[1 - \cos\left(\frac{\pi(t-t_0)}{\Delta_{\mathrm{FWHM}}}\right)\right] \tag{C14b}$$

$$\langle X_{\mathrm{V}}|\mathcal{P}^{(1)}_{t_0\to t}[|X_{\mathrm{V}}\rangle\langle X_{\mathrm{H}}|]|X_{\mathrm{H}}\rangle \approx 2\alpha_H^2\alpha_V^2 + \alpha_H^4 e^{i\pi(t-t_0)/\Delta_{\mathrm{FWHM}}} + \alpha_V^4 e^{-i\pi(t-t_0)/\Delta_{\mathrm{FWHM}}} \tag{C14c}$$

where $j, \ell \in \{H, V\}$ and $\ell \neq j$. Here the propagator $\mathcal{P}^{(1)}_{t_0\to t}$ is used, i.e., the radiative decay of the exciton state is neglected, cf., Eq. (C7). In the following it will become clear that this corresponds to the approximation that no second photon is emitted during the interval $F = \Delta_{\mathrm{FWHM}}$. Note that this assumption in combination with the previous ones results in the feature that the propagation of an exciton occupation or coherence during the interval $F$ can not lead to finite elements outside of the exciton subspace, i.e., $\langle\chi|\mathcal{P}^{(1)}_{t_0\to t}[|X_j\rangle\langle X_{j'}|]|\chi'\rangle = 0$ for $\chi, \chi' \in \{G, B\}$ and $j, j' \in \{H, V\}$.

## III. Two-photon density matrix and concurrence

Based on the estimated dynamics of the statistical operator, we now turn to the integrated two-time correlation functions. With the definitions $t_{s/e} := t_\mathrm{L} \mp \Delta_\mathrm{FWHM}/2$ the expression for the integrated two-time correlation function can be re-formulated as

$$\overline{G}^{(2)}_{jk,\ell m} = \int_0^\infty \mathrm{d}t \int_0^\infty \mathrm{d}\tau\, G^{(2)}_{jk,\ell m}(t,\tau) = \int_{t_s}^\infty \mathrm{d}t \int_0^\infty \mathrm{d}\tau\, G^{(2)}_{jk,\ell m}(t,\tau) = \overline{G}^{(I)}_{jk,\ell m} + \overline{G}^{(II)}_{jk,\ell m} + \overline{G}^{(III)}_{jk,\ell m} \tag{C15a}$$

$$\overline{G}^{(I)}_{jk,\ell m} = \int_{t_s}^{t_e} \mathrm{d}t \int_0^{t_e - t} \mathrm{d}\tau\, G^{(2)}_{jk,\ell m}(t,\tau) \tag{C15b}$$

$$\overline{G}^{(II)}_{jk,\ell m} = \int_{t_s}^{t_e} \mathrm{d}t \int_{t_e - t}^{\infty} \mathrm{d}\tau\, G^{(2)}_{jk,\ell m}(t,\tau) \tag{C15c}$$

$$\overline{G}^{(III)}_{jk,\ell m} = \int_{t_e}^{\infty} \mathrm{d}t \int_0^{\infty} \mathrm{d}\tau\, G^{(2)}_{jk,\ell m}(t,\tau) \tag{C15d}$$

Using the effective model, the respective propagators $\mathcal{P}^{(n)}_{t_0\to t}$ are time-independent, enabling an easier evaluation of $\overline{G}^{(2)}_{jk,\ell m}$. The first contribution can in good approximation be omitted. Due to the very narrow integration intervals for $t$ and $\tau$ on the order of the FWHM $\Delta_\mathrm{FWHM}$, it is much smaller than the other two contributions. Note that omitting this term corresponds to the assumption that the probability for emitting two photons during the effective pulse interval is negligible. For the following calculations we use $F$ instead of $\Delta_\mathrm{FWHM}$ in order to shorten the expressions.

We first evaluate the third term. Note that if the real-time argument $t$ is larger than $t_e$, one only obtains a nonzero contribution when the system is in the biexciton state at this point in time. Starting initially in the ground state, the third term leads to the contribution

$$\begin{aligned}
\overline{G}^{(III)}_{jk,\ell m} &= \int_{t_e}^{\infty} \mathrm{d}t \int_0^{\infty} \mathrm{d}\tau\, G^{(2)}_{jk,\ell m}(t,\tau) = \int_{t_e}^{\infty} \mathrm{d}t \int_0^{\infty} \mathrm{d}\tau\ \mathrm{Tr}\left\{\hat{\sigma}^\dagger_k \hat{\sigma}_m \mathcal{P}^{(0)}_{t\to t+\tau}\left[\hat{\sigma}_\ell \hat{\rho}(t) \hat{\sigma}^\dagger_j\right]\right\} \\
&= \int_{t_e}^{\infty} \mathrm{d}t \int_0^{\infty} \mathrm{d}\tau\ \mathrm{Tr}\left\{\hat{\sigma}^\dagger_k \hat{\sigma}_m \mathcal{P}^{(0)}_{0\to\tau}\left[\hat{\sigma}_\ell \mathcal{P}^{(0)}_{t_e\to t}\left[\langle B|\mathcal{P}^{(2)}_{t_s\to t_e}[|G\rangle\langle G|]|B\rangle\ |B\rangle\langle B|\right]\hat{\sigma}^\dagger_j\right]\right\} \\
&= \int_{t_e}^{\infty} \mathrm{d}t \int_0^{\infty} \mathrm{d}\tau\ \mathrm{Tr}\left\{\hat{\sigma}^\dagger_k \hat{\sigma}_m \mathcal{P}^{(0)}_{0\to\tau}\left[e^{-\gamma_\mathrm{B}F/2} e^{-\gamma_\mathrm{B}(t-t_e)}|X_\ell\rangle\langle X_j|\right]\right\} \\
&= e^{-\gamma_\mathrm{B}F/2}\frac{1}{\gamma_\mathrm{B}} \int_0^{\infty} \mathrm{d}\tau\ \mathrm{Tr}\left\{\hat{\sigma}^\dagger_k \hat{\sigma}_m \mathcal{P}^{(0)}_{0\to\tau}\left[|X_\ell\rangle\langle X_j|\right]\right\} = e^{-\gamma_\mathrm{B}F/2}\frac{1}{\gamma_\mathrm{B}}\delta_{jk}\delta_{\ell m}\frac{1}{\gamma_\mathrm{X} + i(E_\ell - E_j)/\hbar}
\end{aligned} \tag{C16}$$

The evaluation of the last integral is known from Eq. (B6).

Next, the second term is evaluated. Because of the insignificant exciton occupation during the effective pulse interval due to the two-photon resonant excitation character, only two photon states are considered, where the first photon is emitted from the biexciton state. These contributions should clearly dominate over ones where the first photon is emitted from an exciton decay. Thus, we set $\hat{\sigma}_\ell = |X_\ell\rangle\langle B|$ and $\hat{\sigma}^\dagger_j = |B\rangle\langle X_j|$. Furthermore, if an exciton occupation or coherence is propagated during the pulse window, the propagator $\mathcal{P}^{(1)}_{t\to t'}$ is used, cf., Eq. (C14). Thus, the radiative decay of the exciton state is neglected in this short interval. This also corresponds to the assumption that no subsequent second photon is emitted during the pulse window and is justified by the numerical observation

that the concurrence hardly depends on $\gamma_{\mathrm{X}}$ as long as $\gamma_{\mathrm{X}}\Delta_{\mathrm{FWHM}} \ll 1$.

$$\begin{aligned}
\overline{G}^{(II)}_{jk,\ell m} &\approx \int_{t_s}^{t_e} \mathrm{d}t \int_{t_e-t}^{\infty} \mathrm{d}\tau \, \mathrm{Tr}\left\{\hat{\sigma}_k^\dagger \hat{\sigma}_m \mathcal{P}^{(0)}_{t_e\to t+\tau}\left[\mathcal{P}^{(1)}_{t\to t_e}\left[|X_\ell\rangle\langle B|\,\mathcal{P}^{(2)}_{t_s\to t}[|G\rangle\langle G|]\,|B\rangle\langle X_j|\right]\right]\right\} \\
&= \int_{t_s}^{t_e} \mathrm{d}t \int_{t_e-t}^{\infty} \mathrm{d}\tau \, \frac{1}{2}\left(1-\cos[\pi(t-t_s)/F]\right) e^{-\gamma_{\mathrm{B}}(t-t_s)/2}\, \mathrm{Tr}\left\{\hat{\sigma}_k^\dagger \hat{\sigma}_m \mathcal{P}^{(0)}_{t_e\to t+\tau}\left[\mathcal{P}^{(1)}_{t\to t_e}\left[|X_\ell\rangle\langle X_j|\right]\right]\right\} \qquad \text{(C17a)}
\end{aligned}$$

$$\begin{aligned}
\overline{G}^{(II)}_{jj,jj} &= e^{-\gamma_{\mathrm{B}}F/2} \int_{t_s}^{t_e} \mathrm{d}t \int_{t_e-t}^{\infty} \mathrm{d}\tau \, \frac{1}{2}\left(1+\cos[\pi(t-t_e)/F]\right) e^{-\gamma_{\mathrm{B}}(t-t_e)/2}\, e^{-\gamma_{\mathrm{X}}(t+\tau-t_e)} \\
&\qquad \times \left\{1+2\alpha_H^2\alpha_V^2\left(\cos[\pi(t_e-t)/F]-1\right)\right\} \\
&= e^{-\gamma_{\mathrm{B}}F/2}\frac{1}{\gamma_{\mathrm{X}}} \int_{-F}^{0} \mathrm{d}t\, \frac{1}{2}\left(1+\cos[\pi\, t/F]\right) e^{-\gamma_{\mathrm{B}}t/2} \left\{1+2\alpha_H^2\alpha_V^2\left(\cos[\pi\, t/F]-1\right)\right\} \\
&= e^{-\gamma_{\mathrm{B}}F/2}\frac{1}{\gamma_{\mathrm{X}}} \int_{-F}^{0} \mathrm{d}t\, \left(\frac{1}{2}-\alpha_H^2\alpha_V^2\sin^2[\pi\, t/F]+\frac{1}{2}\cos[\pi\, t/F]\right) e^{-\gamma_{\mathrm{B}}t/2} \\
&\approx e^{-\gamma_{\mathrm{B}}F/2}\frac{1}{\gamma_{\mathrm{X}}}\left(\frac{F}{2}-\frac{\alpha_H^2\alpha_V^2 F}{2}\right) e^{\gamma_{\mathrm{B}}F/4} = \frac{F}{2\gamma_{\mathrm{X}}}\left(1-\alpha_H^2\alpha_V^2\right) e^{-\gamma_{\mathrm{B}}F/4} \qquad \text{(C17b)}
\end{aligned}$$

$$\begin{aligned}
\overline{G}^{(II)}_{HH,VV} &= e^{-\gamma_{\mathrm{B}}F/2} \int_{t_s}^{t_e} \mathrm{d}t \int_{t_e-t}^{\infty} \mathrm{d}\tau \, \frac{1}{2}\left(1+\cos[\pi(t-t_e)/F]\right) e^{-\gamma_{\mathrm{B}}(t-t_e)/2}\, e^{-[\gamma_{\mathrm{X}}-i\delta/\hbar](t+\tau-t_e)} \\
&\qquad \times \left\{2\alpha_H^2\alpha_V^2+\alpha_H^4 e^{i\pi(t_e-t)/F}+\alpha_V^4 e^{-i\pi(t_e-t)/F}\right\} \\
&= e^{-\gamma_{\mathrm{B}}F/2}\frac{1}{\gamma_{\mathrm{X}}-i\delta/\hbar} \int_{-F}^{0} \mathrm{d}t\, \frac{1}{2}\left(1+\cos[\pi\, t/F]\right) e^{-\gamma_{\mathrm{B}}t/2} \left\{2\alpha_H^2\alpha_V^2+\alpha_H^4 e^{-i\pi\, t/F}+\alpha_V^4 e^{i\pi\, t/F}\right\} \\
&\approx e^{-\gamma_{\mathrm{B}}F/2}\frac{1}{\gamma_{\mathrm{X}}-i\delta/\hbar}\left(\alpha_H^2\alpha_V^2 F+\frac{\alpha_H^4 F}{4}+\frac{\alpha_V^4 F}{4}\right) e^{\gamma_{\mathrm{B}}F/4} = \frac{F}{2(\gamma_{\mathrm{X}}-i\delta/\hbar)}\left(\frac{1}{2}+\alpha_H^2\alpha_V^2\right) e^{-\gamma_{\mathrm{B}}F/4} \qquad \text{(C17c)}
\end{aligned}$$

$$\begin{aligned}
\overline{G}^{(II)}_{HV,HV} &= e^{-\gamma_{\mathrm{B}}F/2} \int_{t_s}^{t_e} \mathrm{d}t \int_{t_e-t}^{\infty} \mathrm{d}\tau \, \frac{1}{2}\left(1+\cos[\pi(t-t_e)/F]\right) e^{-\gamma_{\mathrm{B}}(t-t_e)/2}\, e^{-\gamma_{\mathrm{X}}(t+\tau-t_e)} \left\{2\alpha_H^2\alpha_V^2\left(1-\cos[\pi(t_e-t)/F]\right)\right\} \\
&= e^{-\gamma_{\mathrm{B}}F/2}\frac{1}{\gamma_{\mathrm{X}}} \int_{-F}^{0} \mathrm{d}t\, \alpha_H^2\alpha_V^2\sin^2[\pi\, t/F] e^{-\gamma_{\mathrm{B}}t/2} \approx \frac{\alpha_H^2\alpha_V^2 F}{2\gamma_{\mathrm{X}}} e^{-\gamma_{\mathrm{B}}F/4} \qquad \text{(C17d)}
\end{aligned}$$

Here, it is assumed that $\gamma_{\mathrm{B}}F/2$ is a small quantity. In this situation one also finds that

$$e^{-\gamma_{\mathrm{B}}F/2}+\frac{\gamma_{\mathrm{B}}F}{2}e^{-\gamma_{\mathrm{B}}F/4} \approx 1 \qquad \text{(C18)}$$

Note that following the same steps one obtains $\overline{G}^{(II)}_{VH,VH} = \overline{G}^{(II)}_{HV,HV}$. Therefore, one ends up with the total integrated correlation functions

$$\begin{aligned}
\overline{G}^{(2)}_{jj,jj} &= \frac{1}{\gamma_{\mathrm{X}}\gamma_{\mathrm{B}}}\left[e^{-\gamma_{\mathrm{B}}F/2}+\frac{\gamma_{\mathrm{B}}F}{2}e^{-\gamma_{\mathrm{B}}F/4}\left(1-\alpha_H^2\alpha_V^2\right)\right] \approx \frac{1}{\gamma_{\mathrm{X}}\gamma_{\mathrm{B}}}\left(1-\alpha_H^2\alpha_V^2\frac{\gamma_{\mathrm{B}}F}{2}e^{-\gamma_{\mathrm{B}}F/4}\right) \qquad \text{(C19a)} \\
\overline{G}^{(2)}_{HH,VV} &= \frac{1}{(\gamma_{\mathrm{X}}-i\delta/\hbar)\gamma_{\mathrm{B}}}\left[e^{-\gamma_{\mathrm{B}}F/2}+\frac{\gamma_{\mathrm{B}}F}{2}e^{-\gamma_{\mathrm{B}}F/4}\left(\frac{1}{2}+\alpha_H^2\alpha_V^2\right)\right] \\
&\approx \frac{1}{(\gamma_{\mathrm{X}}-i\delta/\hbar)\gamma_{\mathrm{B}}}\left[1-\frac{\gamma_{\mathrm{B}}F}{4}e^{-\gamma_{\mathrm{B}}F/4}\left(1-2\alpha_H^2\alpha_V^2\right)\right] \qquad \text{(C19b)} \\
\overline{G}^{(2)}_{HV,HV} &= \frac{1}{\gamma_{\mathrm{X}}\gamma_{\mathrm{B}}}\alpha_H^2\alpha_V^2\frac{\gamma_{\mathrm{B}}F}{2}e^{-\gamma_{\mathrm{B}}F/4} = \overline{G}^{(2)}_{VH,VH} \qquad \text{(C19c)}
\end{aligned}$$

where we employ the approximation given in Eq. (C18). The normalization for the two-photon density matix is thus

$$\mathrm{Tr}\left\{\overline{G}^{(2)}_{jk,\ell m}\right\} = 2\left(\overline{G}^{(2)}_{HH,HH} + \overline{G}^{(2)}_{HV,HV}\right) = \frac{2}{\gamma_\mathrm{X}\gamma_\mathrm{B}} \tag{C20}$$

Finally, the elements of the two-photon density matrix are calculated according to Eq. (A10a):

$$\rho^{2\mathrm{p}}_{HH,HH} = \rho^{2\mathrm{p}}_{VV,VV} = \left(\frac{1}{2} - \alpha_H^2\alpha_V^2\frac{\gamma_\mathrm{B}F}{4}e^{-\gamma_\mathrm{B}F/4}\right) \tag{C21a}$$

$$\rho^{2\mathrm{p}}_{HH,VV} = \frac{1}{1-i\frac{\delta}{\hbar\gamma_\mathrm{X}}}\left[\frac{1}{2} - \frac{\gamma_\mathrm{B}F}{8}e^{-\gamma_\mathrm{B}F/4}\left(1-2\alpha_H^2\alpha_V^2\right)\right] = \left(\rho^{2\mathrm{p}}_{VV,HH}\right)^* \tag{C21b}$$

$$\rho^{2\mathrm{p}}_{HV,HV} = \alpha_H^2\alpha_V^2\frac{\gamma_\mathrm{B}F}{4}e^{-\gamma_\mathrm{B}F/4} = \rho^{2\mathrm{p}}_{VH,VH} \tag{C21c}$$

Using the approximation presented in Eq. (A14) the concurrence can be estimated as

$$C \approx 2\left(|\rho^{2\mathrm{p}}_{HH,VV}| - \rho^{2\mathrm{p}}_{HV,HV}\right) = C_0(\gamma_\mathrm{X},\delta)\left\{1 - f(\gamma_\mathrm{B},F)\left[1+g(\alpha_H)\right]\right\} - f(\gamma_\mathrm{B},F)\left[1-g(\alpha_H)\right] \tag{C22a}$$

$$C_0(\gamma_\mathrm{X},\delta) = \frac{1}{\sqrt{1+\left(\frac{\delta}{\hbar\gamma_\mathrm{X}}\right)^2}} \tag{C22b}$$

$$f(\gamma_\mathrm{B},F) = \frac{\gamma_\mathrm{B}F}{8}\exp\left[-\frac{\gamma_\mathrm{B}F}{4}\right] \tag{C22c}$$

$$g(\alpha_H) = \left(1-2\alpha_H^2\right)^2 \tag{C22d}$$

Thus, the analytic approximation for the concurrence presented in Eq. (6) of the main text is obtained.

## D. DISCUSSION: HORIZONTAL LASER POLARIZATION

In this section we discuss and interpret the influence of a laser pulse with horizontal polarization. A horizontal laser polarization corresponds to setting $\alpha_H = 1$ and $\alpha_V = 0$. In this situation, the approximate result in Eq. (C22) reduces to

$$C = 2|\rho^{2\mathrm{p}}_{HH,VV}| = C_0(\gamma_\mathrm{X},\delta)\left[1 - 2f(\gamma_\mathrm{B},\Delta_\mathrm{FWHM})\right] \tag{D1}$$

and the only four non-zero elements of the two-photon density matrix are the occupations $\rho^{2\mathrm{p}}_{HH,HH} = \rho^{2\mathrm{p}}_{VV,VV} = 1/2$ and the coherence $\rho^{2\mathrm{p}}_{HH,VV} = (\rho^{2\mathrm{p}}_{VV,HH})^*$. Thus, the deviation from a maximally entangled states is caused solely by a reduced coherence. The contribution to this effect, that originates from the influence of the laser pulse can be best understood when looking at the dressed states of the effective model and the approximate time evolution of an exciton occupation and coherence during the pulse duration.

For a horizontal laser polarization the four energy eigenstates of $\hat{H}_1$ are, cf., Eq. (C4),

$$|U\rangle = c\left(|G\rangle + |B\rangle\right) + \sqrt{2}\tilde{c}|X_\mathrm{H}\rangle \approx |X_\mathrm{H}\rangle \tag{D2a}$$

$$|M\rangle = |X_\mathrm{V}\rangle \tag{D2b}$$

$$|N\rangle = \frac{1}{\sqrt{2}}\left(|G\rangle - |B\rangle\right) \tag{D2c}$$

$$|L\rangle = \tilde{c}\left(|G\rangle + |B\rangle\right) - \sqrt{2}c|X_\mathrm{H}\rangle \approx \frac{1}{\sqrt{2}}\left(|G\rangle + |B\rangle\right) \tag{D2d}$$

Since the laser pulse couples only to the transitions between $|X_\mathrm{H}\rangle$ and the ground or biexciton state, the interaction of laser and QD leads to the formation of three dressed states $|U\rangle$, $|N\rangle$, and $|L\rangle$ while the remaining state $|X_\mathrm{V}\rangle$ is unaffected. This dressing effect results in an energetic splitting between the vertically polarized exciton state $|X_\mathrm{V}\rangle$ and the dressed state $|U\rangle$, which for our parameters is essentially the horizontally polarized exciton state, cf., discussion in Section C II. Thus the horizontally polarized exciton state experiences a Stark-shift due to the interaction with the laser. According to Eq. (C12), the energetic splitting between the exciton states is approximately

$$E_\mathrm{S} = E_\mathrm{U} - E_\mathrm{M} \approx \frac{\hbar\pi}{\Delta_\mathrm{FWHM}} \tag{D3}$$

Therefore the laser pulse introduces an effective splitting between the exciton states. After the emission of a first biexciton photon during the pulse window, the QD is in a superposition of the two exciton states. The effective splitting then leads to a phase oscillation of the corresponding exciton coherence. This phase oscillation can be observed in the approximate propagation given in Eq. (C14), which reduces to

$$\mathcal{P}^{(1)}_{t_0\to t}[|X_j\rangle\langle X_j|] \approx |X_j\rangle\langle X_j| \tag{D4a}$$

$$\mathcal{P}^{(1)}_{t_0\to t}[|X_\mathrm{V}\rangle\langle X_\mathrm{H}|] \approx e^{i\pi(t-t_0)/\Delta_\mathrm{FWHM}}|X_\mathrm{V}\rangle\langle X_\mathrm{H}| \tag{D4b}$$

for a horizontal laser polarization. In the measurement process when one integrates correlation functions the integration over this phase oscillation causes a reduced absolute coherence value. In other words, one could also say that the laser introduces a which-path information during its interaction time with the QD, since it causes an effective splitting. Note that for an actual Gaussian pulse, this splitting is a time dependent quantity and scales with $\Omega^2(t)$.

Even in the absence of a fine-structure splitting, i.e. $\delta = 0$, this effect results in a two photon density matrix

$$\rho^\mathrm{2p} = \begin{pmatrix} \frac{1}{2} & 0 & 0 & \frac{1}{2}-f \\ 0 & 0 & 0 & 0 \\ 0 & 0 & 0 & 0 \\ \frac{1}{2}-f & 0 & 0 & \frac{1}{2} \end{pmatrix} \tag{D5}$$

in the basis $\{|HH\rangle, |HV\rangle, |VH\rangle, |VV\rangle\}$ with a corresponding concurrence

$$C = 1 - 2f(\gamma_\mathrm{B}, \Delta_\mathrm{FWHM}) \tag{D6}$$

## E. DISCUSSION: DIAGONAL LASER POLARIZATION

In this section we discuss and interpret the influence of a laser pulse with diagonal polarization. The diagonal laser polarization corresponds to setting $\alpha_H = \alpha_V = 1/\sqrt{2}$. Thus, the general approximate result in Eq. (C22) simplifies to

$$C \approx 2\left(|\rho^\mathrm{2p}_{HH,VV}| - \rho^\mathrm{2p}_{HV,HV}\right) = C_0(\gamma_\mathrm{X},\delta)\left[1 - f(\gamma_\mathrm{B}, \Delta_\mathrm{FWHM})\right] - f(\gamma_\mathrm{B}, \Delta_\mathrm{FWHM}) \tag{E1}$$

and the six most important elements of the two-photon density matrix are the occupations $\rho^\mathrm{2p}_{HH,HH} = \rho^\mathrm{2p}_{VV,VV}$ and $\rho^\mathrm{2p}_{HV,HV} = \rho^\mathrm{2p}_{VH,VH}$ as well as the coherence $\rho^\mathrm{2p}_{HH,VV} = (\rho^\mathrm{2p}_{VV,HH})^*$. In this situation, one obtains the ratio

$$\frac{|\rho^\mathrm{2p}_{HH,VV}|}{\rho^\mathrm{2p}_{HH,HH}} = C_0 \tag{E2}$$

Thus the ratio of the coherence $\rho^\mathrm{2p}_{HH,VV}$ and the occupation $\rho^\mathrm{2p}_{HH,HH}$ is precisely the same as for the initial value calculation presented in Section B. Consequently, the impact of the laser pulse as captured by the function $f$ does not equate to an additional effective splitting that reduces the coherence compared to its corresponding occupations. Instead the reduced degree of entanglement originates from finite occupations $\rho^\mathrm{2p}_{HV,HV}$ and $\rho^\mathrm{2p}_{VH,VH}$, i.e., two-photon states that consist of photons with two different polarizations. Again, the impact of the laser pulse can be analyzed by investigating the dressed states of the effective model and the approximate time evolution of an exciton occupation during the pulse duration.

For a diagonal laser polarization, the four eigenstates of the effective Hamiltonian $\hat{H}_1$, given in Eq. (C4), become

$$|U\rangle = c\left(|G\rangle + |B\rangle\right) + \tilde{c}\left(|X_\mathrm{H}\rangle + |X_\mathrm{V}\rangle\right) \approx \frac{1}{\sqrt{2}}\left(|X_\mathrm{H}\rangle + |X_\mathrm{V}\rangle\right) \tag{E3a}$$

$$|M\rangle = \frac{1}{\sqrt{2}}\left(|X_\mathrm{H}\rangle - |X_\mathrm{V}\rangle\right) \tag{E3b}$$

$$|N\rangle = \frac{1}{\sqrt{2}}\left(|G\rangle - |B\rangle\right) \tag{E3c}$$

$$|L\rangle = \tilde{c}\left(|G\rangle + |B\rangle\right) - c\left(|X_\mathrm{H}\rangle + |X_\mathrm{V}\rangle\right) \approx \frac{1}{\sqrt{2}}\left(|G\rangle + |B\rangle\right) \tag{E3d}$$

In contrast to the horizontal laser polarization, all four states are dressed states, i.e., are a mixture of several bare states. In particular, the two upper dressed states, $|U\rangle$ and $|M\rangle$, are in good approximation equal superpositions of

both exciton states. Just as the lower dressed states $|N\rangle$ and $|L\rangle$ describe the two-photon resonant excitation between the ground and biexciton state (cf., Section C II), the upper ones represent a two-photon resonant process between the two orthogonally polarized exciton states.

This effect is clearly visible in the approximate time dynamics of an exciton state during the pulse interval $F$. For a diagonal laser polarization, Eq. (C14) yields

$$\begin{aligned}\mathcal{P}^{(1)}_{t_0\to t}[|X_j\rangle\langle X_j|] \approx &\frac{1}{2}\left[1+\cos\left(\frac{\pi\,(t-t_0)}{\Delta_{\mathrm{FWHM}}}\right)\right]|X_j\rangle\langle X_j| + \frac{i}{2}\sin\left(\frac{\pi\,(t-t_0)}{\Delta_{\mathrm{FWHM}}}\right)(|X_j\rangle\langle X_\ell| - |X_\ell\rangle\langle X_j|)\\ &+\frac{1}{2}\left[1-\cos\left(\frac{\pi\,(t-t_0)}{\Delta_{\mathrm{FWHM}}}\right)\right]|X_\ell\rangle\langle X_\ell|\end{aligned} \tag{E4}$$

where $j,\ell\in\{H,V\}$ and $\ell\neq j$. This approximate dynamics describes precisely a full-amplitude (coherent) oscillation between the two different exciton states. Thus, if a first biexciton photon is emitted during the pulse duration and the system is in an exciton state, the pulse introduces an effective coupling to the other exciton state. Therefore, the exciton state can change during the pulse duration and the subsequent exciton photon can have a different polarization than the biexciton photon. Consequently, the interaction with the laser, enables the creation of two-photon states $|HV\rangle$ and $|VH\rangle$, which are unwanted and represent a deviation from the maximally entangled state $|\Phi_\pm\rangle$. Hence one obtains a reduced degree of entanglement.

Note that this effective coupling between the exciton states does not include an actual re-excitation back into the biexciton state. Thus no additional photons are created. Still the degree of entanglement drops.

Most importantly, even in the absence of a fine-structure splitting, i.e. $\delta=0$, the effective coupling results in a two-photon density matrix[9]

$$\rho^{2\mathrm{p}} = \begin{pmatrix} \frac{1}{2}(1-f) & 0 & 0 & \frac{1}{2}(1-f)\\ 0 & \frac{1}{2}f & \frac{1}{2}f & 0\\ 0 & \frac{1}{2}f & \frac{1}{2}f & 0\\ \frac{1}{2}(1-f) & 0 & 0 & \frac{1}{2}(1-f)\end{pmatrix} \tag{E5}$$

in the basis $\{|HH\rangle,|HV\rangle,|VH\rangle,|VV\rangle\}$ with a corresponding concurrence

$$C = 1-2f(\gamma_{\mathrm{B}},\Delta_{\mathrm{FWHM}}) \tag{E6}$$

The rise of the elements $\rho^{2\mathrm{p}}_{HV,HV}$ and $\rho^{2\mathrm{p}}_{VH,VH}$ by $f/2$ leads to a reduction of the occupations $\rho^{2\mathrm{p}}_{HH,HH}$ and $\rho^{2\mathrm{p}}_{VV,VV}$ and the corresponding coherence $\rho^{2\mathrm{p}}_{HH,VV}$ by the same amount.

Note that the expression for the concurrence is identical to the result for a vanishing fine-structure splitting using a horizontal laser polarization, given in Eq. (D6). From a physical point of view, this must be fulfilled. For a vanishing fine-structure splitting no pair of orthogonal polarized exciton states is distinguished. Therefore, one could simply perform a basis transformation into a new pair of exciton states

$$|X_{\mathrm{D}}\rangle = \frac{1}{\sqrt{2}}\left(|X_{\mathrm{H}}\rangle + |X_{\mathrm{V}}\rangle\right) \tag{E7a}$$

$$|X_{\mathrm{A}}\rangle = \frac{1}{\sqrt{2}}\left(|X_{\mathrm{H}}\rangle - |X_{\mathrm{V}}\rangle\right) \tag{E7b}$$

where only one exciton ($|X_{\mathrm{D}}\rangle$) couples to the laser polarization and the other is decoupled. Of course after this transformation, the system is identical to the situation of a horizontal laser polarization as discussed in Section D. Consequently the resulting degree of entanglement must also remain the same.

In addition, when one also transforms the measurement basis for the two-photon density matrix accordingly, i.e., from $H$ and $V$ polarization to the diagonal $D$ and anti-diagonal $A$ basis via

$$|D\rangle = \frac{1}{\sqrt{2}}\left(|H\rangle + |V\rangle\right) \tag{E8a}$$

$$|A\rangle = \frac{1}{\sqrt{2}}\left(|H\rangle - |V\rangle\right) \tag{E8b}$$

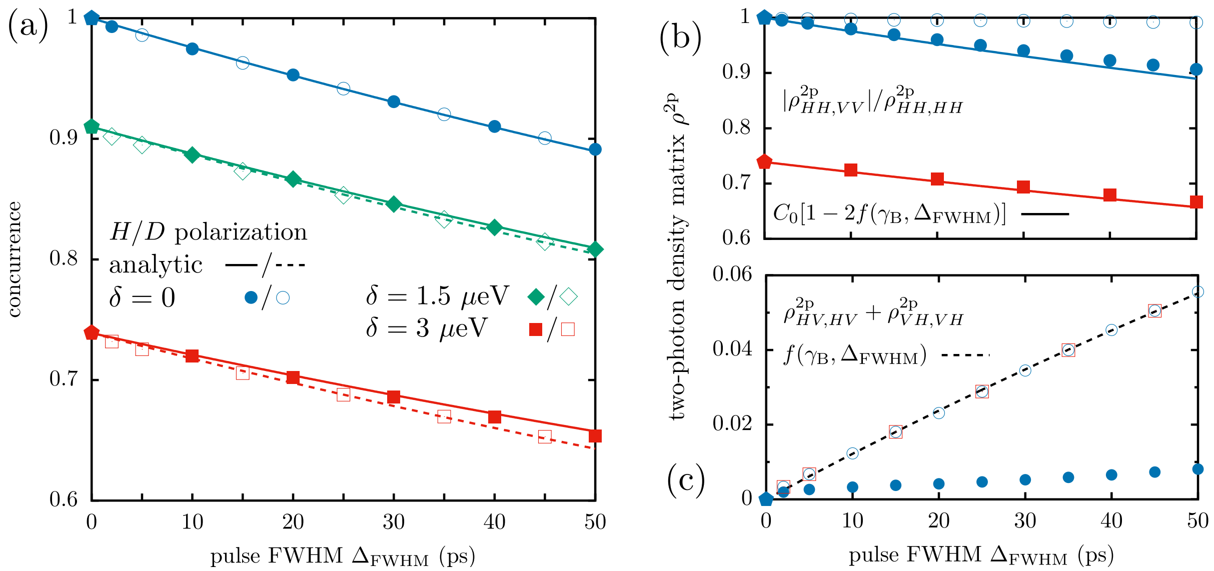


FIG. F1. (a) Concurrence in dependence of the pulse duration, characterized by the FWHM $\Delta_{\rm FWHM}$. Results are shown for two laser polarizations [horizontal ($H$): filled symbols and diagonal ($D$): open symbols] and three fine-structure splittings $\delta = 0$ (blue circles), 1.5 $\mu$eV (green diamonds), and 3 $\mu$eV (red squares). In addition to numerical results (symbols), the analytic approximation according to Eq. (C22) is included as lines with the same color [$H$ ($D$) polarization: solid (dashed) line]. For $\delta = 0$, the results for $H$ and $D$ polarization are exactly the same. Data points at $\Delta_{\rm FWHM} = 0$ (pentagons) represent calculations with an initially prepared biexciton. (b) Ratio between the density matrix elements $\rho^{\rm 2p}_{HH,VV}$ and $\rho^{\rm 2p}_{HH,HH}$ for $\delta = 0$ ($H$ and $D$ polarization) and $\delta = 3\ \mu$eV (only $H$ polarization) together with the analytic estimate for a horizontal laser polarization. (c) Sum of the elements $\rho^{\rm 2p}_{HV,HV}$ and $\rho^{\rm 2p}_{VH,VH}$ for $\delta = 0$ ($H$ and $D$ polarization) and $\delta = 3\ \mu$eV (only $D$ polarization) together with the analytic estimate for a diagonal laser polarization.

the two-photon density matrix becomes

$$\rho^{\rm 2p} = \begin{pmatrix} \frac{1}{2} & 0 & 0 & \frac{1}{2}-f \\ 0 & 0 & 0 & 0 \\ 0 & 0 & 0 & 0 \\ \frac{1}{2}-f & 0 & 0 & \frac{1}{2} \end{pmatrix} \tag{E9}$$

in the basis $\{|DD\rangle, |DA\rangle, |AD\rangle, |AA\rangle\}$. As expected this is precisely the result obtained for a horizontal laser polarization, cf., Eq. (D5). This finding highlights the fact, that for a vanishing fine-structure splitting both laser polarizations are equivalent and that the influence of the laser pulse which introduces an effective splitting in one picture, i.e., horizontal laser polarization, is equivalent to the effective coupling in the other one, i.e., diagonal laser polarization.

Note that we only discussed two limiting cases. For a vanishing fine-structure splitting, any linear laser polarization will result in the same degree of entanglement and the impact of the laser will in general present itself as a combination of both, an effective splitting and an effective coupling, depending on the chosen basis.

## F. EXTENDED FIGURE 2 - DENSITY MATRIX ELEMENTS

Figure F1 is an extension to Fig. 2 in the main text which also includes selected elements of the two-photon density matrix. In addition to the concurrence, also the numerical data for the density matrix elements agrees very well with the analytic estimate. Thus, the behavior of the two-photon density matrix supports the physical picture and interpretation.

For a horizontal laser polarization, the decreasing concurrence with rising FWHM is caused by an energetic splitting $E_{\rm S}$ between the two exciton states $|X_{\rm H}\rangle$ and $|X_{\rm V}\rangle$, which is introduced by the TPE scheme itself. Thus, the main effect of the laser pulse is an additional loss of coherence, cf., filled symbols in panels (b) and (c). Re-excitation of the system, i.e., the creation of additional photons is negligible. This is evident from the filled blue circles in panel (c). The two-photon density matrix elements $\rho^{\rm 2p}_{HV,HV}$ and $\rho^{\rm 2p}_{VH,VH}$, which in the case of a horizontal laser polarization can only be created after re-excitation, are insignificantly small.

On the other hand, a diagonal laser polarization introduces a direct coupling between the two exciton states $|X_{\mathrm{H}}\rangle$ and $|X_{\mathrm{V}}\rangle$, leading to finite elements with two differently polarized photons $\rho^{2\mathrm{p}}_{HV,HV}$ and $\rho^{2\mathrm{p}}_{VH,VH}$, cf., open symbols in panels (b) and (c). Note that for a diagonal laser polarization the increase of these matrix elements is caused by the effective coupling which does not include an actual re-excitation into the biexciton state.

A finite fine-structure splitting $\delta \ll E_{\mathrm{B}}$ hardly impacts the TPE scheme. Thus, for typical fine-structure splittings, the impact of the laser is virtually independent of $\delta$. This is evident in Fig. F1(c), where hardly any change can be observed when one compares the results for $\delta = 0$ (open blue circles) and $\delta = 3$ $\mu$eV (open red squares).

## G. OPTIMAL LASER POLARIZATION

In this section, we discuss the optimal laser polarization. By variation of the coefficient $\alpha_H \in [-1, 1]$ representing the horizontal component of the laser polarization in Eq. (C22), one can determine the optimal laser polarization.

$$\frac{\partial}{\partial \alpha_H} C = f(\gamma_{\mathrm{B}}, \Delta_{\mathrm{FWHM}}) \left[1 - C_0(\gamma_{\mathrm{X}}, \delta)\right] \frac{\partial}{\partial \alpha_H} g(\alpha_H) \tag{G1a}$$

$$\frac{\partial}{\partial \alpha_H} g = 8\alpha_H \left(2\alpha_H^2 - 1\right) \tag{G1b}$$

For a vanishing fine-structure splitting $\delta = 0$ the function $C_0(\gamma_{\mathrm{X}}, \delta)$, which represents the concurrence for an initially prepared biexciton state, is unity. Thus, in accordance with the discussion at the end of Section E, all linear laser polarizations are equivalent and result in the same degree of entanglement.

This of course changes when the fine-structure splitting is finite and one pair of orthogonally polarized exciton states is distinct by the system. In the situation considered here, i.e., $\delta \ll E_{\mathrm{B}}/2$, Eq. (G1) has three simple zeros: $\alpha_H \in \{0, \pm 1/\sqrt{2}\}$. Since $g(\alpha_H = \pm 1) = g(\alpha_H = 0)$, the highest degree of entanglement is obtained when the laser polarization coincides with one of the two distinct exciton states. On the other hand, the emitted photon pairs have the lowest possible degree of entanglement if a diagonal polarization is used, which has equal components in $H$ and $V$ polarization, i.e., if $\alpha_H = \pm 1/\sqrt{2}$. The difference between the maximum and minimum degree of entanglement for a given fine-structure splitting and pulse duration is

$$\begin{aligned} \Delta C &= C(\alpha_H = 0) - C(\alpha_H = 1/\sqrt{2}) \\ &= f(\gamma_{\mathrm{B}}, \Delta_{\mathrm{FWHM}}) \left[1 - C_0(\gamma_{\mathrm{X}}, \delta)\right] \end{aligned} \tag{G2}$$

## H. DIFFERENT PULSE SHAPE: RECTANGULAR PULSE

In this section the impact of the pulse shape is investigated. To this end, we present results for a different pulse shape. The numerical calculations are repeated for a rectangular pulse with smoothened edges where the (real) envelope $\Omega_{\mathrm{R}}(t)$ is given by

$$\Omega_{\mathrm{R}}(t) = \frac{\Omega_0}{\left[1 + e^{-a(t+T/2-t_{\mathrm{L}})}\right]\left[1 + e^{-a(T/2-t+t_{\mathrm{L}})}\right]} \tag{H1}$$

The full-width-at-half-maximum (FWHM) $\Delta_{\mathrm{FWHM}}$ of this rectangular pulse shape is related to the parameter $T$ by

$$\Delta_{\mathrm{FWHM}} = \frac{2}{a} \operatorname{arcosh}\left[2 + \cosh\left(\frac{a\,T}{2}\right)\right] \tag{H2}$$

In the numerical simulation, the parameter $a$, which determines the rise and decay of the pulse, is set to $1/a = 0.25$ ps. In this situation, the FWHM of the rectangular pulse is in good approximation given by the parameter $T$, for all pulse lengths considered in the numerical calculations. The time $t_{\mathrm{L}}$ corresponds to the center of the pulse envelope and the amplitude $\Omega_0$ is determined numerically for each pulse duration such that the biexciton occupation becomes maximal. As an example for a rectangular pulse, the resulting pulse shape for $T = 10$ ps is depicted in Fig. H1(a).

Figure H1(b) shows the concurrence as a function of the pulse duration, characterized by the FWHM, for a rectangular pulse shape as defined in Eq. (H1). In addition we added the analytic results according to Eq. (C22), which are not dependent on the pulse shape, and thus are the same as in Fig. 2 in the main text. Comparing the numerical results for the rectangular pulse to the analytic expression, we also find an excellent agreement, as in the case of

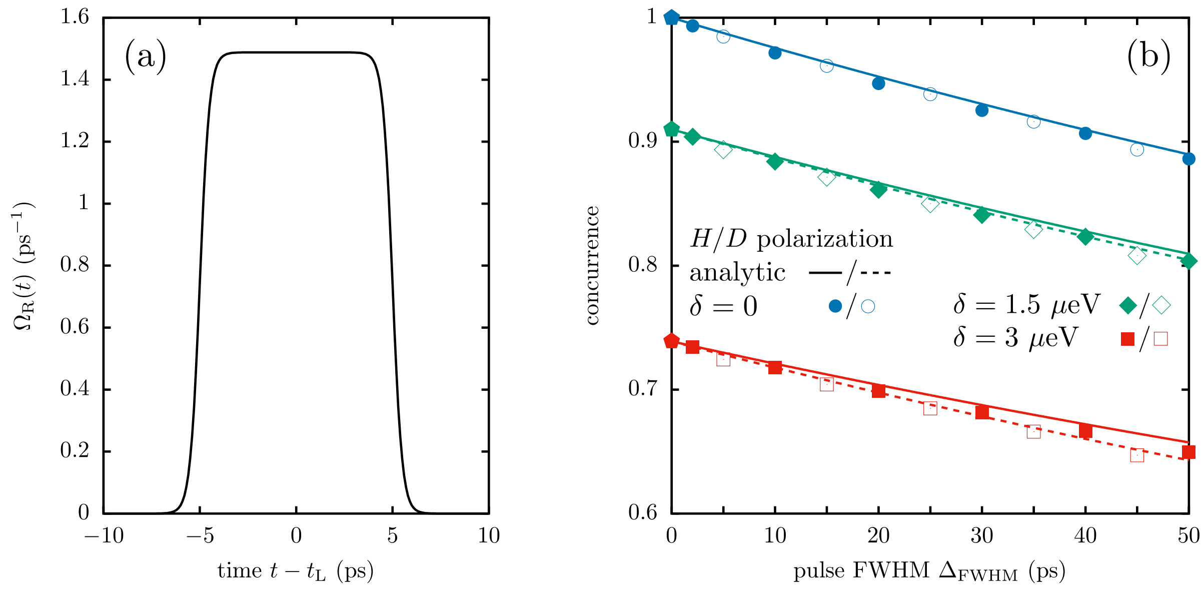


FIG. H1. (a) Rectangular pulse with smoothened edges according to Eq. (H1) for an exemplary pulse duration $T = 10$ ps. The optimal pulse amplitude $\Omega_0 \approx 1.448\,\text{ps}^{-1}$ is determined numerically. (b) Same as Fig. 2 from the main text but for a rectangular pulse shape with FWHM $\Delta_{FWHM}$ according to Eq. (H2). Results are shown for two laser polarizations [horizontal ($H$): filled symbols and diagonal ($D$): open symbols] and three fine-structure splittings $\delta = 0$ (blue circles), 1.5 $\mu$eV (green diamonds), and 3 $\mu$eV (red squares). In addition to numerical results (symbols), the analytic approximation according to Eq. (C22) is included as lines with the same color [$H$ ($D$) polarization: solid (dashed) line]. For $\delta = 0$, the results for $H$ and $D$ polarization are exactly the same. Data points at $\Delta_{FWHM} = 0$ (pentagons) represent calculations with an initially prepared biexciton.

a Gaussian pulse shapes [cf., Fig. 2 or Fig. F1(a)]. A closer inspection shows that the concurrence values for the rectangular pulses are marginally lower than the Gaussian ones. Thus, we conclude that the actual pulse shape has only a weak impact on the concurrence and is of minor importance.

[1] G. Lindblad, Commun. Math. Phys. **48**, 119 (1976).
[2] S. Bravyi, D. P. DiVincenzo, and D. Loss, Ann. Phys. **326**, 2793 (2011).
[3] R. Winkler, *Spin-Orbit Coupling Effects in Two-Dimensional Electron and Hole Systems*, Springer Tracts in Modern Physics, Vol. 191 (Springer, Berlin, 2003).
[4] D. F. V. James, P. G. Kwiat, W. J. Munro, and A. G. White, Phys. Rev. A **64**, 052312 (2001).
[5] M. Cygorek, F. Ungar, T. Seidelmann, A. M. Barth, A. Vagov, V. M. Axt, and T. Kuhn, Phys. Rev. B **98**, 045303 (2018).
[6] M. Cosacchi, M. Cygorek, F. Ungar, A. M. Barth, A. Vagov, and V. M. Axt, Phys. Rev. B **98**, 125302 (2018).
[7] W. K. Wootters, Phys. Rev. Lett. **80**, 2245 (1998).
[8] T. Seidelmann, M. Cosacchi, M. Cygorek, D. E. Reiter, A. Vagov, and V. M. Axt, Adv. Quantum Technol. **4**, 2000108 (2021).
[9] Although not all elements are explicitly derived, this expression for the density matrix is the appropriate result when one uses the effective model and calculation scheme presented in Section C.
